# Supplementary material for: Fragility and Robustness in Mean-Payoff Adversarial Stackelberg Games
Source: arXiv:2007.07209 source file (2021-08-02)
Supplement: Supplementary file 1 [file ZeroSumGames.tex]

\subsection{Two-player zero-sum mean-payoff games} \label{sec:zero-sum}
The zero-sum mean-payoff game is played between two players, Player~0 and Player~1, for an infinite duration and on a finite (single) weighted arena $\mathcal{A} = (V,E, \zug{V_0,V_1}, w)$, where $V$ is a set of vertices partitioned into $V_0$ and $V_1$ belonging to Player~0 and Player~1 respectively, $E$ is a set of edges, and $w: E \rightarrow \mathbb{Q}$ assigns a rational weight to the edges of $\mathcal{A}$.
We denote the zero-sum mean-payoff game by $\mathcal{G}_0 = (\mathcal{A}, \mpgen)$.
Initially, a token is put on some vertex of $\mathcal{G}_0$. At each step of the play, the player controlling the vertex where the token is present chooses an outgoing edge and moves the token along the edge to the next vertex. Players interact in this way an infinite number of times and a play $\pi$ of the game is simply an infinite path traversed by the token.
At each step, the objective of Player~0 is to choose an outgoing edges from the vertices she owns in a way so as to maximise the $\liminf$ of the mean of the play $\pi$, denoted $\underline{\mpgen}(\pi)$, while the objective of Player~1 is the opposite.
Given a rational $c$, the \emph{value} problem in the zero-sum mean-payoff game is to decide whether Player~0 has a strategy to get a mean-payoff greater than $c$ against all possible strategies of Player~1.
Zero-sum mean-payoff games are determined, and optimal memoryless strategies are known to exist for both players \cite{EM79}.
Since zero-sum mean-payoff games are determined, for every vertex $v \in V$ of a zero-sum mean-payoff game $\mathcal{G}_0$, we have that $\sup_{\sigma_0 \in \Sigma_0} \inf_{\sigma_1 \in \Sigma_1} \mpinf(\outv(\sigma_0,\sigma_1)) = \inf_{\sigma_1 \in \Sigma_1} \sup_{\sigma_0 \in \Sigma_0} \mpinf(\outv(\sigma_0,\sigma_1))=\val_{\mathcal{G}_0}(v)$, also called the \emph{value} of the game $\mathcal{G}_0$.
