# Supplementary material for: Fragility and Robustness in Mean-Payoff Adversarial Stackelberg Games
Source: arXiv:2007.07209 source file (2021-08-02)
Supplement: Supplementary file 4 [file compute-eps.tex]

% \subsection{Proof of \cref{thm:ComputeEpsilon}}
% \label{app:ComputeEpsilon}
\begin{proof}
\track{
The proof follows from the proof of \cref{ThmComputeASV}, where in each LP we fix the value of $c$, and replace the optimization function from \textit{maximise} $c$ to \textit{maximise} $\epsilon$.
The maximum value of $\epsilon$ is thus found by considering the maximum $\epsilon$ over all LPs for an SCC reachable from $v$, and then taking the maximum of the $\epsilon$ over all such {\sf SCC}s reachable from $v$.}
\end{proof}
