# Supplementary material for: Fragility and Robustness in Mean-Payoff Adversarial Stackelberg Games
Source: arXiv:2007.07209 source file (2021-08-02)
Supplement: Supplementary file 7 [file appendix_intro.tex]

\section{Summary of our results} \label[appendix]{app:summary}
\begin{table}[h]
\centering
% \scalebox{0.8}{
\begin{tabular}{|c|c|c|c|}
\hline
 &
  Threshold Problem &
  Computing ASV &
  Achievability \\ \hline
\begin{tabular}[c]{@{}c@{}}Adversarial \\ fully rational \\ follower\end{tabular} &
  \begin{tabular}[c]{@{}c@{}}{\color[HTML]{009901} {\sf NP}} \\ \\ {\color[HTML]{0000FE} \textbf{Finite Memory}} \\ {\color[HTML]{0000FE} \textbf{Strategy}} \\ {\color[HTML]{0000FE} \textbf{ [\cref{LemFinMemWitnessASVNonEps}]}} \end{tabular} &
  {\color[HTML]{009901} Theory Of Reals} &
  {\color[HTML]{009901} No} \\ \hline
\begin{tabular}[c]{@{}c@{}}Adversarial\\ bounded rational \\ follower\end{tabular} &
  {\color[HTML]{0000FE} \textbf{\begin{tabular}[c]{@{}c@{}}{\sf NP}\\ \\ Finite Memory \\ Strategy\\ {[}\cref{ThmNpForASV}{]} \end{tabular}}} &
  {\color[HTML]{0000FE} \textbf{\begin{tabular}[c]{@{}c@{}}Theory Of Reals\\  {[}\cref{ThmComputeASV}{]} \\ \\ Solving LP \\ in {\sf EXPTime} \\ {[}\cref{ExpTimeForComputeASV}{]} \end{tabular}}} &
  {\color[HTML]{0000FE} \textbf{\begin{tabular}[c]{@{}c@{}}Yes\\ {[}\cref{ThmAchiev}{]} \\ \\ (Requires Infinite \\ Memory\\  {[}\cref{ThmExNeedInfMem}{]}) \end{tabular}}} \\ \hline
\end{tabular}
% }
\caption{Summary of our results}
\label{tab:results}
\end{table}
The results obtained in this work are in blue, while the results from \cite{FGR20} are in green.
