# Supplementary material for: Fragility and Robustness in Mean-Payoff Adversarial Stackelberg Games
Source: arXiv:2007.07209 source file (2021-08-02)
Supplement: Supplementary file 8 [file appendix_prelims.tex]

\section{Additional Notations and Definitions}
Given an arena $\mathcal{A} =  (V, E, \langle V_0, V_1 \rangle, w_0, w_1)$, we recall that $w_0$ and $w_1$ refer to the weight functions of Player~0 and Player~1 respectively. We refer to $w_0$ and $w_1$ as the weight functions assigning weights to the the \emph{first dimension} and the \emph{second dimension} of an edge respectively.
We assume in the sequel that these weights are given in binary.

The size of the game $\mathcal{G}=(\mathcal{A},\langle \mpinf_0, \mpinf_1\rangle)$, denoted $|\mathcal{G}|$, is the sum of the number of vertices and edges appearing in the arena $\mathcal{A}$.

%  \noindent\textbf{Outcomes} 
%  Given $ \pi = \pi_0\pi_1\dots \in \plays$ and $k \in \mathbb{N}$, the prefix $\pi_0\pi_1\dots\pi_k$ of $\pi$ (resp. suffix $\pi_k\pi_{k+1}\dots$ of $\pi$) is denoted by $\pi_{\leqslant k}$ (resp. $\pi_{\geq k}$).
%  Formally, $\mathbf{Out}_h(\mathcal{G}, \overline{\sigma})$ is the play $\pi$ such that $\pi_{\leqslant|h|-1} = h$ and $\forall k \geqslant |h|-1$ it holds that $\pi_{k+1}=\sigma_i(\pi_{\leqslant k})$ if $\pi_k \in V_i$. 
%  We write $h\leqslant\pi$ whenever $h$ is a prefix of $\pi$.

So far, we have defined the mean-payoff using the $\liminf$. We can also define the mean-payoff using the $\limsup$. Here is the formal definition together with its notation: $\overline{\mpgen}_i(\pi) = \limsup\limits_{k \to \infty} \frac{1}{k}w_i(\pi_{\leqslant k}) $.
We would need $\limsup$ in some of the intermediate steps of our proofs.
The definitions of best-responses and adversarial values can also be defined if we consider $\limsup$ instead of $\liminf$ in the mean-payoff functions.
\begin{comment}
\noindent\textbf{Best-Responses} Let $\mathcal{G} = (\mathcal{A},\langle \mpinf_0, \mpinf_1\rangle)$ be a 
% $(\mp_0, \mp_1)$-game 
two-dimensional mean-payoff
on the bi-weighted arena $\mathcal{A}$. Given a strategy $\sigma_0$ for Player~0, we define two sets of strategies for Player~1:
\begin{enumerate}
\item his best-responses to $\sigma_0$, denoted by $\brgen(\sigma_0)$, and defined as:
\begin{equation*}
    \begin{split}
        \{\sigma_1 \in \Sigma_1 & \mid \forall v \in V \cdot \forall \sigma'_1 \in \Sigma _1: \\
        &\quad \mpinf_1(\outv(\sigma_0,\sigma_1)) \geqslant \mpinf_1(\outv(\sigma_0,\sigma'_1))\}
    \end{split}
\end{equation*}
\item his $\epsilon$-best-responses to $\sigma_0$, for $\epsilon > 0$, denoted by $\br(\sigma_0)$, and defined as:
\begin{equation*}
    \begin{split}
        \{\sigma_1 \in & \Sigma_1  \mid \forall v \in V \cdot \forall \sigma'_1 \in \Sigma _1: \\
        &\quad \mpinf_1(\outv(\sigma_0,\sigma_1)) > \mpinf_1(\outv(\sigma_0,\sigma'_1)) - \epsilon\}
    \end{split}
\end{equation*}
\end{enumerate}
Note that for the $\epsilon$-best-response when $\epsilon > 0$, we use $>$ instead of $\geqslant$. 
% \track[FOSSACS]{This change in inequality makes the $\asv$ value achievable, as shown in \cref{sec:Achievability}.}
The above definitions of best-responses and adversarial values can also be defined if we consider $\limsup$ instead of $\liminf$ in the mean-payoff functions.
\end{comment}

\noindent\textbf{Witnesses for $\asvgen$} For a mean-payoff game $\mathcal{G}$, we associate with each vertex $v$ in $\mathcal{G}$, the following set of pairs of real numbers:
% \begin{equation*}
$\Lambda(v) = \{(c,d) \in \mathbb{R}^2 \mid v \vDash \ll 1 \gg \mpinf_0 \leqslant c \land \mpinf_1 \geqslant d \}$.
% \end{equation*}
A vertex $v$ is said to be $(c,d)$-bad if $(c,d) \in \Lambda(v)$. Let $c' \in \mathbb{R}$. A play $\pi$ in $\mathcal{G}$ is called a $(c',d)$-witness of $\asvgen(v) > c$ if $(\mpinf_0(\pi), \mpinf_1(\pi)) = (c', d)$ where $c' > c$, and $\pi$ does not contain any $(c,d)$-bad vertex. A play $\pi$ is called a witness of $\asv(v) > c$ if it is a $(c',d)$-witness of $\asvgen(v) > c$ for some $c',d$. 

% \noindent\textbf{Plays and simple cycles}
% Given a play $\pi \in \plays$, we denote by $\inf(\pi)$ the set of vertices $v$ that appear infinitely many times along $\pi$, i.e., $\inf(\pi) = \{v \in V \mid \forall in \in \mathbb{N}\cdot \exists j \in \mathbb{N}, j \geqslant i: \pi(j) = v \}$. It is easy to see that $\inf(\pi)$ forms an SCC in the underlying graph of the arena $\mathcal{A}$. A \textit{cycle} $c$ is a sequence of edges that starts and stops in a given vertex $v$, it is simple if it does not contain repetition of any other vertex. 

\noindent\textbf{Unfolding of a game}
Let $V$ and $E$ be respectively the set of vertices and the set of edges of $\mathcal{G}$.
The \emph{unfolding} of the game $\mathcal{G}$ starting from a vertex $v \in V$ is a tree $T_v(\mathcal{G})$ of infinite depth with its root $v$ such that there is a one-to-one correspondence between the set of plays $\pi$ of $\mathcal{G}$ with $\first(\pi)=v$ and the branches of $T_v(\mathcal{G})$.
% Every node $v_1$ of $T_v(\mathcal{G})$ belongs to $V$, and there is an edge from $v_1$ to $v_2$ in $T_v(\mathcal{G})$ iff $(v_1, v_2) \in E$.
Every node $p \in V^{+}$ of $T_v(\mathcal{G})$ is a play $p=v_1 \dots v_n$ in $\mathcal{G}$, where $v_1=v$.
There is an edge from $p=v_1 \dots v_n$ to $p'= v_1 \dots v_n v'_n$ iff $(v_n, v'_n) \in E$.
